# Supplementary material for: The Shift Toward Open and Reproducible AI Research
Source: arXiv:2606.16974 source file (2026-06-26)
Supplement: Supplementary file 1 [file supplement.tex]

\input{preamble}

\begin{document}

\title[Supplementary Information]{Supplementary Information: The embrace of open science: An analysis of a decade of AI research 
and 56\,800 conference papers}
\maketitle

\renewcommand{\figurename}{Supplementary Figure} % for captions
\renewcommand{\figureautorefname}{Supplementary Figure} % for \autoref
\renewcommand{\tablename}{Supplementary Table}        % caption prefix
\renewcommand{\tableautorefname}{Supplementary Table} % \autoref output
\renewcommand{\thesection}{S\arabic{section}}


\input{supplement-content}

\clearpage
\bibliography{sn-bibliography}

\end{document}
